# Supplementary material for: Linear Causal Disentanglement via Interventions
Source: arXiv:2211.16467 source file (2023-06-11)
Supplement: Supplementary file 1 [file additional-experiments.tex]

\section{Additional Experimental Results}\label{appendix:additional-experiments}

We
