# Supplementary material for: Linear Causal Disentanglement via Interventions
Source: arXiv:2211.16467 source file (2023-06-11)
Supplement: Supplementary file 2 [file worst-case-observational-alternative.tex]

\section{An algebraic proof of \rref{prop:worst-case-necessity-observed}}\label{appendix:worst-case-observational-alternative}

\begin{proof}
We have $\Theta_k = P_\sigma^\top B_k^\top B_k P_\sigma$ for some permutation $\sigma$.
Let \cbs{TODO: CHECK SIGNS. Can we typeset so that the structure of the matrix is more clear?}
\[
\hatB_k = \begin{bmatrix}
 & - & (B_k)_{1:(p-2),1:p} & - &
\\
0 & \ldots & 0 & \frac{(B_k)_{p-1,p}}{(B_k)_{p,p}} + \frac{(B_k)_{p,p}}{(B_k)_{p-1,p}} & \frac{(B_k)_{p-1,p-1}}{(B_k)_{p,p}}
\\
0 & \ldots & 0 & 0 & \frac{(B_k)_{p-1,p-1}}{(B_k)_{p-1,p}}
\end{bmatrix}
\]
Then we have
\[
\hatB_k^\top \hatB_k
=
\begin{bmatrix}
(B_k^\top B_k)_{1:(p-2),1:(p-2)}
\end{bmatrix}
\]
Suppose $p-1, p \not\in \{ i_k \}_{k=1}^K$.
\end{proof}
